# Supplementary material for: Hidden Markov Model Identifiability via Tensors
Source: arXiv:1305.0321 source file (2013-05-02)
Supplement: Supplementary file 1 [file appendix.tex]

\appendices{}
\section{Useful Lemmas}
\label{app:useful}

We collect results useful in proving our main results in this section.

\subsection{Properties of the row tensor product}
\label{ssec:row_tensor}

The following result collects some useful results on Kruskal's rank. 
\begin{lem}
Let $\bA$ and $\bB$ be real $q\times p$ and $q \times r$ matrices respectively and assume $\krank(\bA) \ge 1$ and $\krank(\bB) 
\ge 1$. Some properties of the row tensor product are as follows:
\begin{enumerate}
\item $\bA \orow \bB = (\bB \orow \bA)\cdot \Perm$ where $\Perm$ is a $pr \times pr$ permutation matrix,
\item $\krank(\bA \orow \bB) = \krank(\bB \orow \bA)$,
\item for any integer $K \ge 1$, $\krank(\bigorow{j=1}{K} \bA_j) \ge \krank(\bigotimes^{K} \bA_j)$, for matrices $\bA_j \in \Real^{q \times r_j}$, and
\item for any integer $K \ge 1$, $\krank(\bigorow{{}}{K} \bB) \ge \krank(\bB)$.
\end{enumerate}
\label{lem:krank_properties}
\end{lem}

\medskip
\noindent
\textbf{Proof of (i)}: Observe that
\begin{align*}
\bA \orow \bB &= 
\begin{bmatrix}
\ba_1 \otimes \bb_1\\
\ba_2 \otimes \bb_2\\
\vdots\\
\ba_q \otimes \bb_q
\end{bmatrix} = 
\begin{bmatrix}
\bb_1 \otimes \ba_1 \Perm_1\\
\bb_2 \otimes \ba_2 \Perm_2\\
\vdots\\
\bb_q \otimes \ba_q \Perm_q
\end{bmatrix}\\
&= (\bB \orow \bA) \cdot \Perm,
\end{align*}
where $\Perm = \diag(\lbrack \Perm_1,\Perm_2,\cdots,\Perm_q\rbrack)$, and $\Perm_j$, $j=1,2,\cdots,q$ are permutation 
matrices. Since each column (and row) of $\Perm$ forms the canonical Euclidean basis in $\Real^{pr}$, then $\Perm$ itself is a 
permutation matrix.

\medskip
\noindent
\textbf{Proof of (ii)}: Suppose there is a non-null column vector $\bx \in \Real^q$ such that $\bx^\T (\bA \orow \bB) = \mnull$ 
and $\krank(\bA \orow \bB) = |\supp(\bx)|-1$. By statement (i), since $\bx^\T (\bA \orow \bB) = \bx^\T(\bB \orow \bA)\cdot 
\Perm = \mnull$, and $\Perm$ is full rank, so $\bx^\T(\bB \orow \bA)= \mnull$, this implies $\krank(\bB \orow \bA) = |\supp(\bx)|-1 
= \krank(\bA \orow \bB)$.

\medskip
\noindent
\textbf{Proof of (iii)}: The case is clearly true for $K=1$. Consider a fixed $K \ge 2$. Let $\bx \in \Real^q$ such that $\bx^\T 
(\bigorow{j=1}{K} \bA_j) = \mnull$ and $\krank(\bigorow{j=1}{K} \bA_j) = |\supp(\bx)|-1$. Observe that the rows of $\bigorow{j=1}
{K} \bA_j$ are a subset of rows in $\bigotimes^{K} \bA_j$. Then, we can construct a vector $\mathbf{\tilde x} \in \Real^{qr_1 
r_2\cdots r_K}$ containing $\supp(\bx)$, such that $\mathbf{\tilde x}^\T (\bigotimes^{K} \bA_j) = \mnull$, by selecting the linearly 
dependent rows in $\bigorow{j=1}{K} \bA_j$. We can perform this construction for any vector that forms linearly dependent 
combinations of rows of $\bB \orow \bA$, as long as the support size is at least $\krank(\bigorow{j=1}{K} \bA_j)+1$. This implies $
\krank(\bigorow{j=1}{K} \bA_j) \ge \krank(\bigotimes^{K} \bA_j)$, since the number linearly dependent rows in the Kronecker 
product $\bigotimes^{K} \bA_j$ must be at most the number of linearly dependent rows in $\bigorow{j=1}{K} \bA_j$. Intuitively, the 
rows of $\bigotimes^{K} \bA_j$ have a greater degree of freedom in their combinations. The same argument applies for any 
value of $K \ge 2$.

\medskip
\noindent
\textbf{Proof of (iv)}: The statement is true for $K=1$. By statement (iii), for any $K \ge 2$, $\krank(\bigorow{{}}{K} \bB) 
\ge \krank(\bigotimes^{K} \bB)$. By the result \cite[Theorem 3.1]{Jokar09KronCS}, $\krank(\bigotimes^{K} \bB) = \krank(\bB)$, 
since $\spark(\bX) = \krank(\bX)+1$ for any matrix $\bX$. The result then follows.

\subsection{Minimality of the HMM}

\begin{lem}
If the minimal representation of the HMM is $q$ hidden states, then $\krank(\bA) = q$.
\label{lem:minimal_states}
\end{lem}
\begin{proof}
We only need to consider the case $\krank(\bA) < q$ since $\krank(\bA)$ cannot exceed $q$. We proceed by contradiction. 
Suppose the HMM is minimal but $\krank(\bA)  < q$, which means at least 
one state in the Markov chain is redundant since the particular state can be expressed in terms of a linear combination of 
other states. Thus, the HMM is not minimal, resulting in a contradiction.   
\end{proof}

\section{Proof of Main Results}
\label{app:main}

In this section, we collect the proofs of all results presented in the paper.

\subsection{Proof of Lemma \ref{lem:row_tensor_krank}}

The proof is exactly like the proof of the Kruskal rank of the Khatri-Rao product in \cite{Sidiropoulos99Tensor}. We reproduce
the proof here, with appropriate modifications, for completeness.

Let $s$ be the smallest number of linearly dependent rows drawn from $\bB \orow \bA$. These rows are denoted by
$\bb_{i_1} \otimes \ba_{i_1}, \bb_{i_2} \otimes \ba_{i_2}, \cdots, \bb_{i_s} \otimes \ba_{i_s}$. If a collection of linearly 
dependent columns cannot be found, then by convention, $s = q + 1$. Then, there exists nonzero real scalars $\mu_1,\mu_2,
\cdots, \mu_s$ such that
\ben
\mu_1 \bb_{i_1} \otimes \ba_{i_1} + \mu_2 \bb_{i_2} \otimes \ba_{i_2} + \cdots + \mu_s \bb_{i_s} \otimes \ba_{i_s} = \mnull.
\een
Equivalently, the above may be written as
\be
\bar{\bA}^\T \diag(\lbrack \mu_1, \mu_2,\cdots, \mu_s\rbrack) \bar{\bB} = \mnull,
\label{eq:dependent}
\ee
where
\ben
\bar{\bA} = 
\begin{bmatrix}
\ba_{i_1}\\
\ba_{i_2}\\
\vdots\\
\ba_{i_s}
\end{bmatrix},\ 
\bar{\bB} = 
\begin{bmatrix}
\bb_{i_1}\\
\bb_{i_2}\\
\vdots\\
\bb_{i_s}
\end{bmatrix}.
\een

Using Sylvester's rank inequality \cite[Section 0.4.5]{Horn09Matrix}, we have
\begin{align}
\nonumber
r &:= \rank(\bar{\bA}^\T \diag(\lbrack \mu_1, \mu_2,\cdots, \mu_s\rbrack) \bar{\bB}) \\
\label{eq:rank_inequality}
&\ge \rank(\bar{\bA}^\T) + \rank(\bar{\bB}) - s. 
\end{align}
Moreover, by definition of Kruskal rank,
\begin{align*}
\rank(\bar{\bA}^\T) &= \rank(\bar{\bA}) \ge \min(\krank(\bA),s),\\ 
\rank(\bar{\bB}) &\ge \min(\krank(\bB),s),
\end{align*}
leading to
\ben
r \ge \min(\krank(\bA),s) +  \min(\krank(\bB),s) - s.
\een
Observe that $\min(\krank(\bA) + \krank(\bB) -1,q) \ge \max(\krank(\bA),\krank(\bB))$, since:
\begin{enumerate}
\item if $\krank(\bA) + \krank(\bB) - 1 > q$, then 
\begin{align*}
&\hspace{-0.5cm}\min(\krank(\bA) + \krank(\bB) -1,q) = q \\
&\hspace{0.5cm}\ge \max(\krank(\bA),\krank(\bB)),
\end{align*}
\item else if $\krank(\bA) + \krank(\bB) - 1 \le q$, then 
\begin{align*}
&\hspace{-0.5cm}\min(\krank(\bA) + \krank(\bB) -1,q)\\ &= \krank(\bA) + \krank(\bB) - 1 \\
&= \max(\krank(\bA),\krank(\bB)) \\
&\hspace{0.5cm}+ \min(\krank(\bA),\krank(\bB))-1\\
&\ge~\max(\krank(\bA),\krank(\bB)),
\end{align*} 
since $\krank(\bA),\krank(\bB) \ge 1$.
\end{enumerate}

We now have to consider the different cases for equation \eqref{eq:rank_inequality}:
\begin{enumerate}
\item if $1 \le s \le  \min(\krank(\bA),\krank(\bB))$, then \eqref{eq:rank_inequality} implies $r \ge s \ge 1$,
\item else if $\min(\krank(\bA),\krank(\bB)) < s < \max(\krank(\bA),\krank(\bB))$, then \eqref{eq:rank_inequality} implies 
$r \ge \min(\krank(\bA),\krank(\bB)) + s-s = \min(\krank(\bA),\krank(\bB)) \ge 1$,
\item else if $\max(\krank(\bA),\krank(\bB)) \le s \le \min(\krank(\bA) + \krank(\bB) -1,q)$, then \eqref{eq:rank_inequality} 
implies $r \ge \krank(\bA) + \krank(\bB) -s$; but $s \le \min(\krank(\bA) + \krank(\bB) -1,q)$ implies that $ \krank(\bA) +
\krank(\bB) - 1 \ge s$, and so  $\krank(\bA) + \krank(\bB)-s \ge 1$, thus, $r \ge 1$.
\end{enumerate}
All cases conclude that $r \ge 1$ for $s \le \min(\krank(\bA) + \krank(\bB) -1,q)$. However, $r$ is the rank of 
$\bar{\bA}^\T \diag(\lbrack \mu_1, \mu_2,\cdots, \mu_s\rbrack) \bar{\bB}$, which, from \eqref{eq:dependent}, is a zero 
matrix, and therefore has rank 0. This is a contradiction, which implies that the number of linearly dependent rows drawn
from $\bB \orow \bA$ must strictly exceed $\min(\krank(\bA) + \krank(\bB) -1,q)$.

For the cases when either one or both of $\krank(\bA), \krank(\bB)$ is 0, recall that $\krank(\bA) =0$ if and only if $\bA$ 
contains at least one identically zero row, which means $\bB \orow \bA$ has at least one identically zero row as well,
implying a Kruskal rank of 0. The same argument holds for the case $\krank(\bB) = 0$.

\subsection{Proof of Lemma \ref{lem:single_letter}}

Crucial to our argument is the central claim that it is necessary and sufficient that none of the non-trivial linear 
combinations of rows of $\bB \orow \bA$ is expressible by a tensor product of two row vectors, that is, $\krank(\bB \orow 
\bA) = q$. Necessity is proven by contradiction. We borrow a counterexample from \cite{Jiang04PermLemma}. If 
the first two rows can be expressed as a vector
\ben
\bb_1 \otimes\ba_1 + \bb_2 \otimes \ba_2 = \tb_1 \otimes \ta_1,
\een
then we can obtain an alternative decomposition of $\bcL$ as follows:
\begin{align}
\nonumber
\id{q} \cdot (\bB \orow \bA) &= 
\begin{bmatrix}
1 & -1 & \mathbf{0}\\
0 & 1 & \mathbf{0}\\
\mathbf{0} & \mathbf{0} & \id{q-2}
\end{bmatrix}
\cdot
\begin{bmatrix}
\tb_1 \otimes \ta_1\\
\bb_2 \otimes \ba_2\\
\vdots\\
\bb_q \otimes \ba_q
\end{bmatrix}\\
\label{eq:alternative_decomp}
&= \tC^\T \cdot (\tB \orow \tA).
\end{align}
Since the per letter $\bcL$ is equivalent to $\tC^\T \cdot (\tB \orow \tA)$, there is no unique decomposition for $\bcL$.

The sufficiency of the statement is even easier to establish, since it is easy to show that $\id{q}$ satisfies Kruskal's 
permutation lemma. We only need to verify $|\supp(\bx)| \le |\supp(\tC\bx)|$ for all $|\supp(\tC\bx)| = 1$ (since $\bx =\mnull$ is the 
only zero support vector) for some $\tC$, a component of an alternative decomposition of $\bcL$. With an alternative 
decomposition $\id{q} \cdot (\bB \orow \bA) = \tC^\T \cdot (\tB \orow \tA)$, then $\forall \bx$,
\ben
\bx^\T (\bB \orow \bA) = \bx^\T\tC^\T  (\tB \orow \tA).
\een
Consider $\bx$ with $|\supp(\tC \bx)| = 1$. Then, $\bx^\T\tC^\T  (\tB \orow \tA)$ is just a scaled tensor product of one row of $\tA$ 
and the corresponding row of $\tB$, by the above equation. Thus, $|\supp(\bx)| \le 1$, or the full
Kruskal rank condition of $\bB \orow \bA$ will be violated. Kruskal's permutation lemma (Lemma \ref{lem:kruskal_perm})
then implies $\id{q}$ and $\tC$ are equivalent up to a permutation and scaling of rows.
Putting these arguments together implies the components of $\bcL$, i.e.~$\bA$, $\bB$ and $\id{q}$ are all unique up to a 
permutation and scaling of rows, and the result follows.

\subsection{Proof of Theorem \ref{thm:equivalence}}

Implication (i) follows directly from Kruskal's theorem, since $\bA$ and $\bB$ are unique up to a scaling and permutation of
rows, thus, so would its row-wise product $\bB \orow \bA$ inherit this property.
For implication (ii), the condition of Lemma \ref{lem:single_letter} implies $\krank(\bA) + \krank(\bB) -1 \ge q$, 
which then implies $\krank(\bB \orow \bA) \ge q$, by Lemma \ref{lem:row_tensor_krank}. Since $\krank(\bB \orow \bA) \le 
\rank(\bB \orow \bA) \le \min(q,\kappa q) = q$, this implies $\krank(\bB \orow \bA) = q$. 

We proceed to prove implication (iii) constructively. Firstly, we can always construct matrices $\bPhi$ and $\bPsi$ of size 
$q \times \tilde q$ and $\tilde q \times q$ respectively such that $\bPhi \bPsi = \id{q}$. For example, if $\tilde q \ge q$, we can choose
\ben
\bPhi = \lbrack \bU^\T \ \bV \rbrack, \bPsi = 
\begin{bmatrix}
\bU\\
\bW 
\end{bmatrix}
\een
where $\bU$ is an orthogonal matrix, so $\bU^\T\bU = \id{q}$, while $\bV \bW = \mathbf{0}$, that is, the columns of $\bW$ lie in 
the null space of $\bV$. We can similarly do this for $\tilde q < q$.

By Lemma \ref{lem:single_letter}, then for permutation matrix $\Perm$ and scaling matrices $\Scale_{\bA},\Scale_{\bB}$, we can 
construct a tensor with components $\Perm \Scale_{\bA} \bA$, $(\Perm \Scale_{\bA}\Scale_{\bB})^{-1}$ and $\Perm \Scale_{\bB} 
\bB$. Let $\Scale = \Scale_{\bA} \Scale_{\bB}$, then clearly $\tB \orow \tA = \Perm \Scale (\bB \orow \bA)$. Hence, one can form 
the relations
\begin{align*}
\tpi &= \bpi (\Perm \Scale)^{-1} \bPhi,\\ 
\tilde \bM(k)  &=  \bPsi (\Perm \Scale) \bD_k(\bB) \bA (\Perm \Scale)^{-1} \bPhi, k = 1,2,\cdots \kappa,\\
\tones{\tilde q} &= (\Perm \Scale) \ones{q}.
\end{align*}
Thus, we have formed an HMM with a new parameter set $\tlambda$. Then, it is easy to show both HMMs have the same 
observation probabilities for all sequences, satisfying Definition \ref{def:equivalence}. The result follows by setting $\bX = (\Perm 
\Scale)^{-1} \bPhi$ and $\bY = \bPsi (\Perm \Scale)$.

\subsection{Proof of Theorem \ref{thm:unique_identifiability}}

Recall from equation \eqref{eq:sequence_prob}, the probability of any arbitrary observation sequence $\by$ 
is a function of the matricisation of the per letter tensor $\bcL$. Thus, we only need to focus on $\bcL$, since it is 
assumed $\bpi$ is fully positive.  Lemma \ref{lem:single_letter} shows that if $\krank(\bB \orow \bA)=q$ the per letter 
tensor $\bcL$ is permutation and scaling indeterminate. This proves sufficiency. 

For necessity, we prove by contradiction. Suppose we claim that there exists a unique decomposition for $\bcL$ when $\krank(\bB \orow \bA) < q$. However, if the condition is not satisfied, then there does not exist a unique decomposition for 
$\bcL$. We can construct an equivalent HMM using the example from Lemma \ref{lem:single_letter}, with 
\begin{align*}
\bpi &= \tpi \tC^\T,\\
(\bB \orow \bA) \bE(k)  &=  (\tB \orow \tA) (\bE(k)\tC^\T), \forall k,\\
\ones{q} &= (\tC^\T)^{-1}\tones{q},
\end{align*}
where
\ben
(\tB \orow \tA) = 
\begin{bmatrix}
\bb_1 \otimes\ba_1 + \bb_2 \otimes \ba_2\\
\bb_2 \otimes \ba_2\\
\vdots\\
\bb_q \otimes \ba_q
\end{bmatrix},
\een
and
\ben
\tC = 
\begin{bmatrix}
1 & 0 & \mathbf{0}\\
-1 & 1 & \mathbf{0}\\
\mathbf{0} & \mathbf{0} & \id{q-2}
\end{bmatrix},
\een
applicable to any observation sequence $\by$. But we have claimed that $\bcL$ has a unique decomposition and therefore we arrive 
at a contradiction. Thus, the result is proven.

\subsection{Proof of Theorem \ref{thm:identifiability_measurements}}

In order to prove our result, we rewrite the joint distribution of a stationary HMM parameterised by $\blambda$, $\full$ as
\be
\full =\bpi \bA(\bB \orow \bR),
\label{eq:full_rewrite}
\ee
where $\bR := (\cdots \bA(\bB \orow(\bA(\bB \orow \bA\bB))) \cdots)$. In this way, $\full$ is the sum of the matricisation of a 3-way 
tensor with components $\lbrack \bA^\T, \bB, \bR\rbrack$. The initial state probabilities $\bpi$ are assumed positive, otherwise, 
the HMM can be rewritten with $\tilde q < q$ states. 

We prove our claim in two stages. In the first stage, we first prove generic conditions on the 
identifiability of the components $\lbrack \bA^\T, \bB, \bR\rbrack$. Once that is done, we then need to show that $\bpi$ can
be generically identified, i.e.~the joint distribution of the observation states contain sufficient information to ensure uniqueness of 
$\bpi$.

We generically assume $\bA$ has full row and column rank so that $\krank(\bA^\T) = q$ and $\bA^\T$ is full rank. In 
order for each component to be scaling and permutation indeterminate, it is necessary and sufficient that $\krank(\bB \orow \bR) 
= q$, since this tensor is also a restricted CP model, with similar properties to a per letter tensor $\bcL$. Therefore, the necessary 
and sufficient condition is that none of the nontrivial combinations of rows of $\bB \orow \bR$ results in another row, which may 
be shown using the arguments in the proof of Lemma \ref{lem:single_letter} (see also \cite{Jiang04PermLemma}). 

Our goal is to then show $\bB \orow \bR$ is generically full rank. This will be achieved by showing the vanishing 
polynomials of the determinant of $\bB \orow \bR$ lie in a set of Lebesgue measure zero. We will need the
following result, from \cite{Jiang01Harmonic,Stoica89MUSIC}.
\begin{lem}
Consider an analytic function $h(\bx)$ of several real variables $\bx \in \Real^{n}$. If $h$ is nontrivial in the sense that 
there exists $\bx_0 \in \Real^n$ such that $h(\bx_0) \ne 0$, then the zero set of $h(\bx)$,
\ben
\cZ := \{ \bx \in \Real^n\,|\,h(\bx) = 0\}
\een
has measure zero, in the Lebesgue measure in $\Real^n$.
\label{lem:analytic}
\end{lem}

By the above lemma, it is enough to show $\bB \orow \bR$ has a nonzero minor determinant for one submatrix, for some specific 
choice of $\bpi$, $\bA$ and $\bB$, as it would establish the full rank property of $\bB \orow \bR$. We begin by choosing arbitrary 
$\bpi$ and generically choose $\bA = \id{q}$, which is a valid choice, as it lies within the Zariski closure of the restricted CP 
model. Then, with this generic choice, $\bB \orow \bR = \bigorow{{}}{N} \bB$.

Following the proof of \cite[Theorem 6]{Allman09Latent}, we generically choose $\bB$ to be a Vandermonde matrix with 
$\kappa$ generators $\balpha = \lbrack \alpha_1,\alpha_2,\cdots,\alpha_{\kappa}\rbrack$, such that
\ben
\bB(\balpha) =
\begin{bmatrix}
1 & 1 & \cdots & 1\\
\alpha_1 & \alpha_2 & \cdots & \alpha_\kappa\\
\alpha^2_1 & \alpha^2_2 & \cdots & \alpha^2_\kappa\\
\vdots & \vdots & \ddots & \vdots\\
\alpha^{q-1}_1 & \alpha^{q-1}_2 & \cdots & \alpha^{q-1}_\kappa\\
\end{bmatrix}
\een
since the rank of $\bigorow{{}}{N} \bB$ would not be affected by nonzero rescalings of the rows of $\bB$, and therefore the
rows of $\bB$ do not have to sum to 1 for this choice. 

We only need to show that the polynomial $h(\balpha)$ is nonzero for an arbitrary selection of $q \times q$ submatrix of
$\bigorow{{}}{N} \bB$ implying that its determinant is nonzero. We further define
\begin{align*}
h(\balpha) &= \det\Big(W(\bigorow{{}}{N} \bB(\balpha))\Big),
\end{align*}
where $W(\bX)$ selects an arbitrary $q \times q$ submatrix from $\bX$. Clearly, $h(\balpha)$ is a polynomial in $\kappa$ 
variables and therefore analytic.

Proceeding with the proof, we draw $\kappa$ distinct prime numbers using a probability distribution covering $\Real^\kappa$ 
and assign them to each element of $\balpha$. Then, following the proof of \cite[Theorem 6]{Allman09Latent}, $\bigorow{{}}{N} 
\bB$ is now simply the first $q$ rows of the Vandermonde matrix with generators from the vector $\bigotimes^N \balpha$. To 
show $h(\balpha)$ is nonzero with this choice of $\bB$, it is sufficient for at least $q$ of the elements $\bigotimes^N \balpha$ to 
be distinct, so as to ensure $\bigorow{{}}{N} \bB$ has nonsingular $q \times q$ submatrices. The number of distinct 
elements in the vector $\bigotimes^N \balpha$ corresponds to the number of distinct monomials of degree $N$ in $
\alpha_1,\alpha_2,\cdots,\alpha_{\kappa}$, which is $\tbinom{N+\kappa-1}{\kappa-1}$ in total. We require at least $q$ distinct 
elements, and hence it is then sufficient for $N$ to satisfy
\be
\binom{N+\kappa-1}{\kappa-1} \ge q,
\label{eq:binomial_condition}
\ee
for $\rank(\bigorow{{}}{N} \bB) = \krank(\bigorow{{}}{N} \bB) = q$, almost surely. The minimum number of consecutive 
observations is given by $N^*$, the smallest integer to satisfy \eqref{eq:binomial_condition}. Then, invoking Lemma \ref
{lem:analytic}, the zero set $h(\balpha)$ has Lebesgue measure zero in $\Real^\kappa$. Therefore, the components $\lbrack 
\bA^\T, \bB, \bR\rbrack$ can almost surely be identified from any equivalent parameterisation $\tA := \bA (\Scale_\bB \Scale_\bR)
^{-1} \Perm^\T$, $\tB := (\Scale_\bB \Perm) \bB$ and $\tR := (\Scale_\bR \Perm) \bR$ for some nonsingular scaling and 
permutation matrices $\Scale_\bA$, $\Scale_\bB$ and $\Scale_\bR$, with $\Scale_\bA \Scale_\bB \Scale_\bR = \id{q}$ and 
$\Perm$ respectively.

Finally, to identify $\bpi$, we first need to consider if $\bpi$ is unique. Suppose there exists $\tpi \ne \bpi$ such that
\begin{align*}
\bpi \bA(\bB \orow \bR) = \tpi \bA(\bB \orow \bR)\\
\hspace{5mm} \Rightarrow (\bpi - \tpi) \bA(\bB \orow \bR) = \mnull.
\end{align*}
But by the generic choices,  $ \bA(\bB \orow \bR)$ has full row rank, therefore, the equation implies $\tpi = \bpi$ resulting in
a contradiction. Thus, $\bpi$ is uniquely represented.

Second, we need to now consider if $\bpi$ can be recovered up to a scaling and permutation. 
Consider an equivalent parameterisation of the HMM with $\tlambda$ such that
\begin{align*}
\bpi \bA(\bB \orow \bR) = \tpi \tA(\tB \orow \tR).
\end{align*}
By the choice of $N^*$, $\bA(\bB \orow \bR)$ is generically full row rank, and we know that any equivalent parameterisation
is simply a scaled and permuted version of $\bA$, $\bB$ and $\bR$. Since the Kruskal rank remains unchanged by the 
permutation and scaling of rows, then any $\tpi = \bpi \Scale \Perm$ for some nonsingular scaling and permutation matrix 
$\Scale$ and $\Perm$ respectively, is identifiable as the rows of $\bA(\bB \orow \bR)$ are linearly independent.

This means the joint distribution of the observations contains sufficient information on the uniqueness of $\bpi$, up to a scaling 
and permutation. Thus, by these generic choices, the joint probability of the $N^*$ consecutive observations completely 
describes $\blambda$.

\smallskip
\begin{rem}
The arguments presented in the proof is to fundamentally establish a full Kruskal rank of $\bA(\bB \orow \bR)$. Then, this would
ensure $\bpi$ is uniquely preserved, since none of the rows of $\bA(\bB \orow \bR)$ can be formed from nontrivial 
combinations of the other rows. In fact, the final part of the proof on the identification of $\bpi$ is reminiscent of the identification of 
mixture distributions \cite{Teicher67Mixture,Yakowitz68Mixtures}, in which a necessary and sufficient condition is the linear 
independence of the probability density functions included in the mixture. Each row $1 \le k \le q$ of the matrix $\bA(\bB \orow 
\bR)$ is equivalent to the probability mass function of the observation observations conditioned on $X_1 = k$, essentially enabling 
one to view $\full$ as a mixture of these components. The generic choices were made such that full row rank of $\bA(\bB \orow 
\bR)$ holds, therefore satisfying this fundamental necessary and sufficient condition for mixture distributions.
\end{rem}

\smallskip
\begin{rem}
An alternative but slightly weaker proof relies on Kruskal's sufficient condition in Theorem \ref{thm:kruskal_suff}, where we 
have the condition
\ben
\krank(\bA) + \krank(\bB) + \krank(\bR) \ge 2q + 2.
\een
Using the same generic choices in the above proof with $\krank(\bA) =q$ and $\krank(\bB) \ge 2$, we obtain $\krank(\bR) \ge 
q$. Following the same arguments outlined above, using a generic choice of $\bB$ as a Vandermonde matrix with distinct prime 
number generators, we arrive at a sufficient condition 
\be
\binom{N+\kappa-2}{\kappa-1} \ge q,
\label{eq:weaker_identifiability}
\ee
since $\bR$ is a row tensor product of $N-1$ $\bB$ matrices. To illustrate how this condition is weaker than the above result, 
with a choice $\kappa = 2$, it can be seen that \eqref{eq:weaker_identifiability} results in $N^* \ge q$, while 
\eqref{eq:binomial_condition} results in the condition $N^* \ge q-1$, requiring one less observation.
\end{rem}

\subsection{Proof of Lemma \ref{lem:multi_observer_letter_hetero}}

The proof is similar to the proof of Lemma \ref{lem:single_letter}, extended to the multidimensional case, thus, we only need 
to sketch the proof here. We claim that it is necessary and sufficient that none of the non-trivial linear combinations of 
rows of $\bigorow{j=1}{m} \bB^{(j)} \orow \bA$ is expressible by a tensor product of two row vectors, 
i.e.~$\krank(\bigorow{j=1}{m} \bB^{(j)} \orow \bA) = q$. The chief ingredients are, (1) show a counterexample to proof
necessity, where the same example from the proof of Lemma \ref{lem:single_letter} can be used, appropriately modified to
account for additional dimensions, to construct an alternative decomposition of $\bcM_{\ast}$, and (2) for sufficiency, show
that $\id{q}$, the full rank component of $\bcM_{\ast}$ satisfies Kruskal's permutation lemma. Then, the claim is established.
 
\subsection{Proof of Lemma \ref{lem:multi_observer_letter_homo}}
\label{app:multi_observer_letter_homo}

Consider the case with $m=2$ independent homogeneous observers. We first show why $\krank(\bB) \ge 2$ is necessary, 
using arguments from \cite{Stegeman05Perm}. Clearly, if $\krank(\bB) = 0$, then there is a some component of $
\bcM_{\circ}$ is zero, so at least one row of $\bA$ can be arbitrary vectors. 

Let $\bee_k$ denote the $k$-th Euclidean basis vector in $\Real^q$. Suppose now $\krank(\bB) = 1$, implying that there are at 
least two proportional rows in $\bB$. Let the proportional rows be $\bb_i = \alpha \bb_j$. Then, the sum of the $i$-th and $j$-th 
components is
\begin{align*}
&\ba_i \otimes \bee_i \otimes \bb_i \otimes \bb_i + \ba_j \otimes \bee_j \otimes \bb_j \otimes \bb_j \\
&= \ba_i \otimes \bee_i \otimes \bb_i \otimes \bb_i + \ba_j \otimes \bee_j \otimes \alpha \bb_i \otimes \alpha \bb_i\\
&= \underbrace{(\ba_i \otimes \bee_i + \alpha^2\cdot \ba_j \otimes \bee_j)}_{\bG} \otimes \bb_i \otimes  \bb_i.
\end{align*}
The components of $\bG$ can be written as
\ben
\lbrack
\ba_i\  \alpha^2 \ba_j
\rbrack
\begin{bmatrix}
\bee_i\\
\bee_j
\end{bmatrix}
=
\lbrack
\ba_i\  \alpha^2 \ba_j
\rbrack
\bU
\cdot
\lbrack
\bee_i \  \bee_j
\rbrack^\T
(\bU^{-1})^\T,
\een
with $\bU$ a $2 \times 2$ nonsingular matrix expressing the mixtures between the $i$-th and $j$-th rows of $\bA$ and $\id{q}$. 
The matrix $\bU$ need not be a product of a permutation and diagonal scaling matrix, thus, no unique decomposition for $\bcM_
{\circ}$ can be found. By induction, we can extend this argument to higher dimensions, proving that if $\krank(\bB) < 2$,
there is no unique decomposition for $\bcM_{\circ}$. In the same way, we can also show $\krank(\bA) \ge 2$ is a necessary 
condition.

Essentially, as evident from the proof of Lemma \ref{lem:multi_observer_letter_hetero}, the necessary and sufficient 
condition is $\krank(\bigorow{{}}{m} \bB \orow \bA) = q$. We claim that $\krank(\bB \orow \bA) = q$ if and only if 
$\krank(\bigorow{{}}{m} \bB \orow \bA) = q$. 

To prove sufficiency, using Lemma \ref{lem:row_tensor_krank}, we have
\begin{align*}
&\krank( \bigorow{{}}{m} \bB \orow \bA) \ge \min\Big(\krank(\bB\orow\bA)\\
 &\hspace{0.5cm} + \krank(\bigorow{{}}{m-1} \bB)-1,q \Big) \ge q,
\end{align*}
since $\krank(\bB\orow\bA) = q$ and $\krank(\bigorow{{}}{m-1} \bB) \ge \krank(\bB) \ge 1$, by Lemma 
\ref{lem:krank_properties}(iv) and $\krank(\bigorow{{}}{m} \bB \orow \bA) \le q$.

We proceed by a contradiction to prove necessity. Suppose $\krank(\bB \orow \bA) = q$ and $\krank( \bigorow{{}}{m} \bB 
\orow \bA) < q$. Then, $\bcM_{\circ}$ is not unique up to a permutation and scaling, so there exists an alternative
decomposition similar to a multidimensional generalisation of equation \eqref{eq:alternative_decomp}, with component matrices 
$\tA$, $\tB$ and $\tC$. We can then form a subarray equivalent to the per letter tensor $\bcL$, such that $\id{q} \cdot (\bB \orow 
\bA) = \tC^\T \cdot (\tB \orow \tA)$. Since there is an alternative decomposition of $\bcL$ not due to a permutation and scaling 
matrix, thus, there does not exist a unique decomposition with permutation and scaling indeterminacy for $\bcL$ as well, 
implying $\krank(\bB \orow \bA) < q$. This implies a contradiction, and the result follows.

Finally, recall that $\krank(\bB \orow \bA) = q$ effectively implies $\krank(\bA),\,\krank(\bB) \ge 2$, since the condition implies that
neither $\bA$ nor $\bB$ has a pair of proportional rows.

%where in \eqref{eq:inequality_B}, we have $\krank(\bigorow{{}}{m} \bB) = \krank(\bB)$ by Lemma 
%\ref{lem:krank_properties}(iii). Thus, the necessary and sufficient condition reduces to $\krank(\bA) + \krank(\bB)-1 \ge q$,
%which is equivalent to Lemma \ref{lem:single_letter} for the single letter tensor $\bcL$.

%By Lemma \ref{lem:row_tensor_krank},
%\begin{align}
%\nonumber
%\krank( \bigorow{{}}{m} \bB \orow \bA) &\ge \min(\krank(\bA) + \krank(\bigorow{{}}{m} \bB)-1,q)\\
%\label{eq:inequality_B}
%&= \min(\krank(\bA) + \krank(\bB)-1,q),
%\end{align}
%where in \eqref{eq:inequality_B}, we have $\krank(\bigorow{{}}{m} \bB) = \krank(\bB)$ by Lemma 
%\ref{lem:krank_properties}(iii). Thus, the necessary and sufficient condition reduces to $\krank(\bA) + \krank(\bB)-1 \ge q$,
%which is equivalent to Lemma \ref{lem:single_letter} for the single letter tensor $\bcL$.

\subsection{Proof of Lemma \ref{lem:row_tensor_krank_multi}}

First, assume that for all $j=1,2,\cdots,K$, $\krank(\bA_j) \ge 1$. We prove the result by induction, starting from case $k=1$. The 
case $k=1$ is clearly true. The case $k=2$ is true, since  $\krank(\bA_2 \orow \bA_1) \ge \min(\krank(\bA_1) + \krank(\bA_2)-1,q)
$ is true by Lemma \ref{lem:row_tensor_krank}. 

Assume the result is true for case $k \ge 2$. Then, for case $k+1$, without loss of generality (by the property (ii) of
row tensor products in Appendix \ref{ssec:row_tensor}), we have ordered the matrices in a sequence $\bA_{k+1}, \bA_{k},
\cdots, \bA_{1}$ in the row tensor product, and so
\begin{align*}
&\krank(\bA_{k+1} \orow \bA_{k} \orow \cdots \orow \bA_{1})\\
&\ge \min\Big(\krank(\bA_{k+1}) \\
&\hspace{0.5cm} + \krank(\bA_{k} \orow \cdots \orow \bA_{1})-1, q \Big)\\
&\ge \min\Big(\krank(\bA_{k+1}) \\
&\hspace{0.5cm}+ \min(\sum_{j=1}^k \krank(\bA_{j})-k+1,q)-1, q \Big),
\end{align*}
by application of Lemma \ref{lem:row_tensor_krank} and the assumption that the case is true in case $k$. If $\sum_{j=1}^k 
\krank(\bA_{j})-k+1 \ge q$, then the right side reduces to $\min(\krank(\bA_{k+1})+q-1, q) = q$, since $\krank(\bA_{k+1}) 
\ge 1$; otherwise, $\min(\krank(\bA_{k+1}) + \sum_{j=1}^k \krank(\bA_{j})-k, q)$ is obtained instead, where the expression
checks if addition with the term $\krank(\bA_{k+1})$ exceeds $q$ or not. In either case, the inequality is true for case $k+1$,
proving the result.

It remains to show what happens in the case when there is one $\bA_{j'}$ such that $\krank(\bA_{j'})=0$. Since 
$\krank(\bA_{j'})=0$ if and only if at least one row of $\bA_{j'}$ is a row of zeros, then, the row tensor product 
$\krank(\bigorow{j=1}{K} \bA_j) = 0$ since the product will also have at least one row of zeros, and the result follows.

\subsection{Proof of Theorem \ref{thm:measurements_homo}}

We sketch a proof using arguments from the proof of Theorem \ref{thm:identifiability_measurements}. In the homogeneous multi 
observer case, since each observer is independent to the others, each observation is i.i.d.~with $\kappa$ states per observer. 
We generically choose an arbitrary positive $\bpi$, full row rank $\bA$ by setting $\bA = \id{q}$, and $\bB$ to be 
a Vandermonde matrix with $\kappa$ distinct prime numbers as its generators, denoted by $\balpha = \lbrack \alpha_1, 
\alpha_2, \cdots, \alpha_\kappa \rbrack$. 

The matrix $\bigorow{{}}{m\cdot N} \bB$ has its $q$ rows equivalent to the first $q$ rows of a Vandermonde matrix with 
generators from $\bigotimes^{m\cdot N} \balpha$. To enforce full rank of this submatrix, we require the number of 
distinct monomials of degree $m\cdot N$ to exceed $q$, resulting in the sufficient condition,
\ben
\binom{N\cdot m+\kappa-1}{\kappa-1} \ge q,
\een
The rest of the proof follows the proof of Theorem \ref{thm:identifiability_measurements}
 
\subsection{Proof of Theorem \ref{thm:measurements_hetero}}

We sketch a proof following arguments from the proof of Theorem \ref{thm:identifiability_measurements}. We generically choose
an arbitrary positive $\bpi$, full row rank $\bA$ by setting $\bA = \id{q}$, and for each $j = 1,2,\cdots,m$, 
\ben
\bB^{(j)}(\balpha_j) =
\begin{bmatrix}
1 & 1 & \cdots & 1\\
\alpha_{j,1} & \alpha_{j,2} & \cdots & \alpha_{j,\kappa_j}\\
\alpha^2_{j,1} & \alpha^2_{j,2} & \cdots & \alpha^2_{j,\kappa_j}\\
\vdots & \vdots & \ddots & \vdots\\
\alpha^{q-1}_{j,1} & \alpha^{q-1}_{j,2} & \cdots & \alpha^{q-1}_{j,\kappa_j}\\
\end{bmatrix},
\een
Vandermonde matrices with distinct generators $\balpha_j = \lbrack \alpha_{j,1},\alpha_{j,2},\cdots,\alpha_{j,\kappa_j}\rbrack$. 

Let
\begin{align*}
h(\balpha_1,\balpha_2, \cdots, \balpha_m) 
= \det\Big(W(\bigorow{{}}{N} \bigorow{j=1}{m}\bB^{(j)}(\balpha_j))\Big),
\end{align*}
where $W(\bX)$ selects an arbitrary $q \times q$ submatrix from $\bX$, as before and $h(\balpha_1,\balpha_2, \cdots, 
\balpha_m) $ is a polynomial in $\kappa'$ variables and therefore analytic. In order to show that there exists a nonvanishing $q 
\times q$ minor, we draw $\kappa'$ distinct prime numbers from $\Real^{\kappa'}$ and assign them to the generators 
$\balpha_j$ for each $j$. 

The matrix $\bigorow{{}}{N} \bigorow{j=1}{m}\bB^{(j)}(\balpha_j))$ has its $q$ rows equivalent to the first $q$ rows of a 
Vandermonde matrix with generator $\bigotimes^N \bigotimes_{j=1}^m \balpha_j$. Since the number of distinct elements in the 
vector $\bigotimes^N \bigotimes_{j=1}^m \balpha_j$ corresponds to the number of distinct monomials of degree $N\cdot m$ in 
the $\kappa'$ generators, we require $N$ to satisfy
\ben
\binom{N\cdot m+\kappa'-1}{\kappa'-1} \ge q,
\een
so that $\rank(\bigorow{{}}{N} \bigorow{j=1}{m}\bB^{(j)}(\balpha_j)) = \krank(\bigorow{{}}{N} \bigorow{j=1}{m}\bB^{(j)}(\balpha_j)) 
= q$, almost surely. Invoking Lemma \ref{lem:analytic}, the zero set $h(\balpha)$ has Lebesgue measure zero in 
$\Real^{\kappa'}$. The rest of the proof follows the proof of Theorem \ref{thm:identifiability_measurements}.
